# Supplementary material for: Nanomagnetic Self-Organizing Logic Gates
Source: arXiv:2012.12721 source file (2020-12-23)
Supplement: Supplementary file 1 [file Suppl_DynamicalAnalysis.tex]

We will simulate the sLLG dynamics (\ref{eq:sLLG}) of each proposed NAND gate design following two distinct protocols to evaluate consistency. The first protocol, which we will term {\it free-floating}, will allow the gates to evolve under the combined effects of thermal noise, magnetic interactions and no applied currents such that each non-fixed island magnetization will randomly switch as a result of these processes. We will assign (or not) a logical label $\lambda_q$ to the gate by observing the sign of the terminal island's perpendicular magnetization components at each moment in time. This allows us to compute the time spent by the gate in each allowed logical state and, as a result, estimate both $LC$ and $WB$. The second protocol, which we will term {\it clocked}, will periodically apply an in-plane polarized current pulse to each island to effectively reset all non-fixed islands and successively allowing them to relax again. The relaxation timescale setting the current periodicity is chosen to be smaller than the average switching timescale observed in the first protocol. At the end of each clocking cycle we assign a logical label to the gate's state and collect $LC$/$WB$ statistics over a large number of repetitions. This second protocol more closely emulates previous NML experiments where clocking fields are used to force gates to reset their magnetic states. The choice of these two protocols is two-fold. The first will assess gate robustness to successive spin-flip events while the second will assess robustness on individual relaxation events.

Figures~\ref{fig:DynOptimalA},~\ref{fig:DynOptimalB}, and ~\ref{fig:DynOptimalC} show the results obtained from the simulation of these two protocols. What immediately stands out is how the logical Boltzmann probabilities and, consequently, $LC$/$WB$ measures are very different from those obtained through the statical analysis of the previous section. This demonstrates how influential the evolution of the stray-fields as a result of dynamical transients can be. More specifically, the effectiveness of thermal noise at precluding the individual islands from ever exactly being in an $m_{i,z}=\pm 1$ state strongly invalidates expectations from the previous section. The results shown can however be considered significantly useful in the sense that both protocols produce statistics which are in strong agreement.   

\begin{figure}
	\centerline{\includegraphics[width=6in]{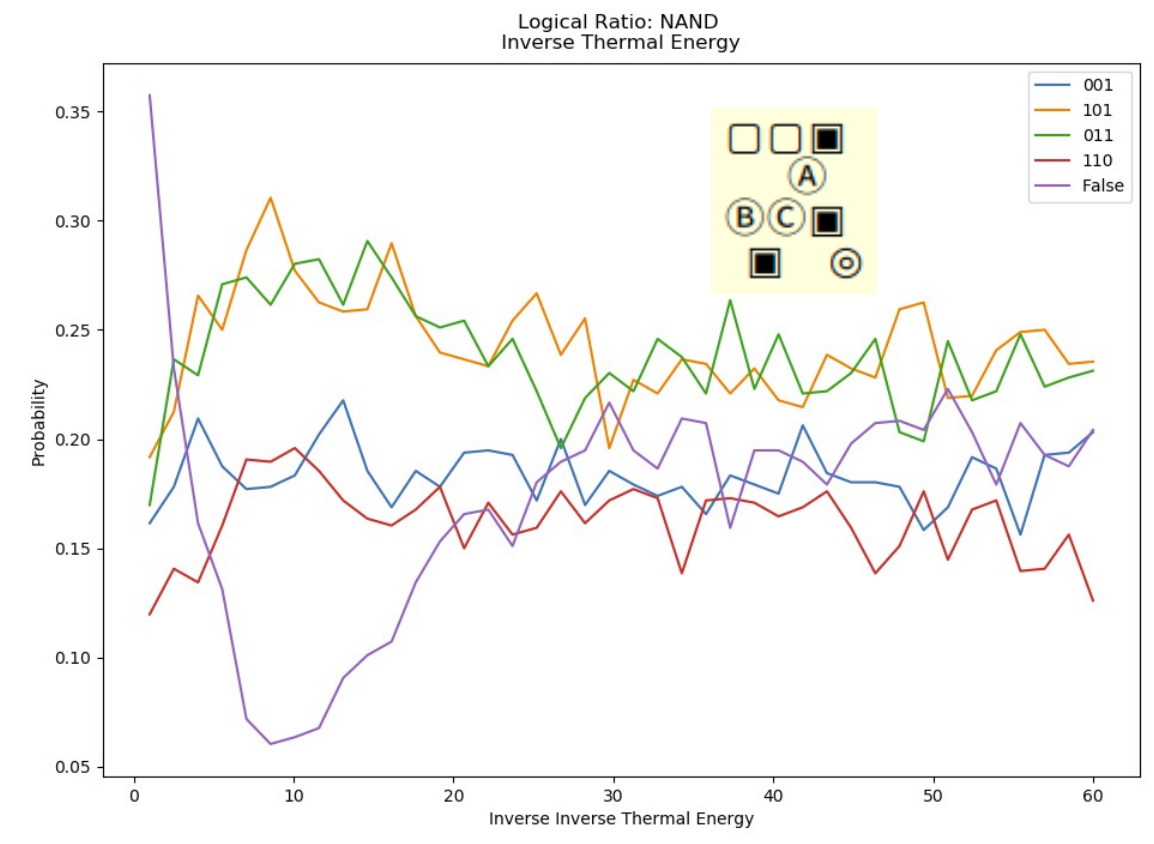}}
	\caption{{\footnotesize BlaBla.}}
	\label{fig:DynOptimalA}
\end{figure} 

\begin{figure}
	\centerline{\includegraphics[width=6in]{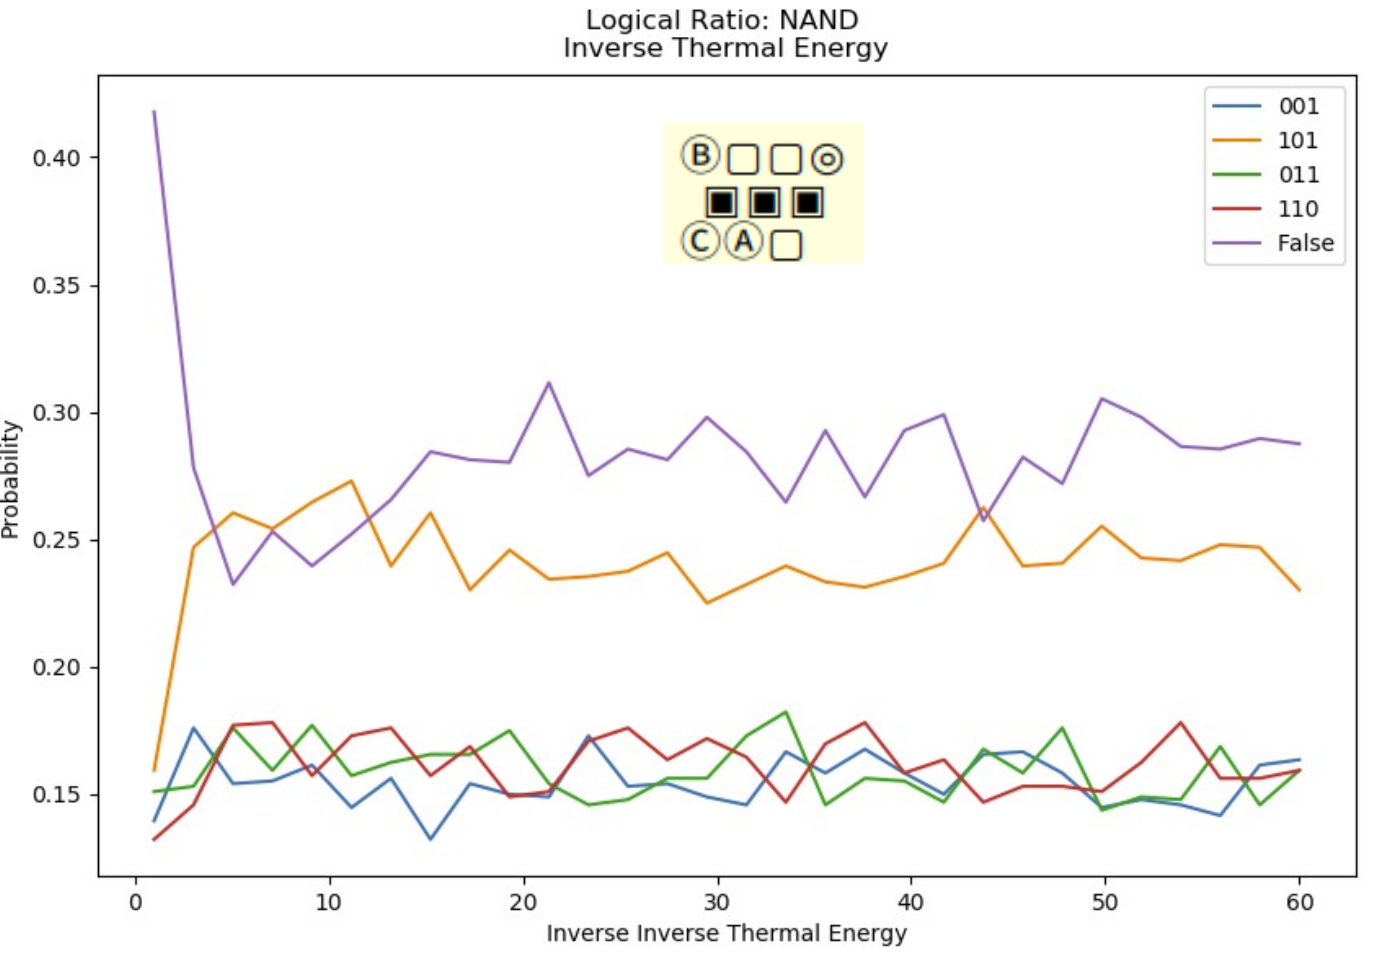}}
	\caption{{\footnotesize BlaBla.}}
	\label{fig:DynOptimalB}
\end{figure} 

\begin{figure}
	\centerline{\includegraphics[width=6in]{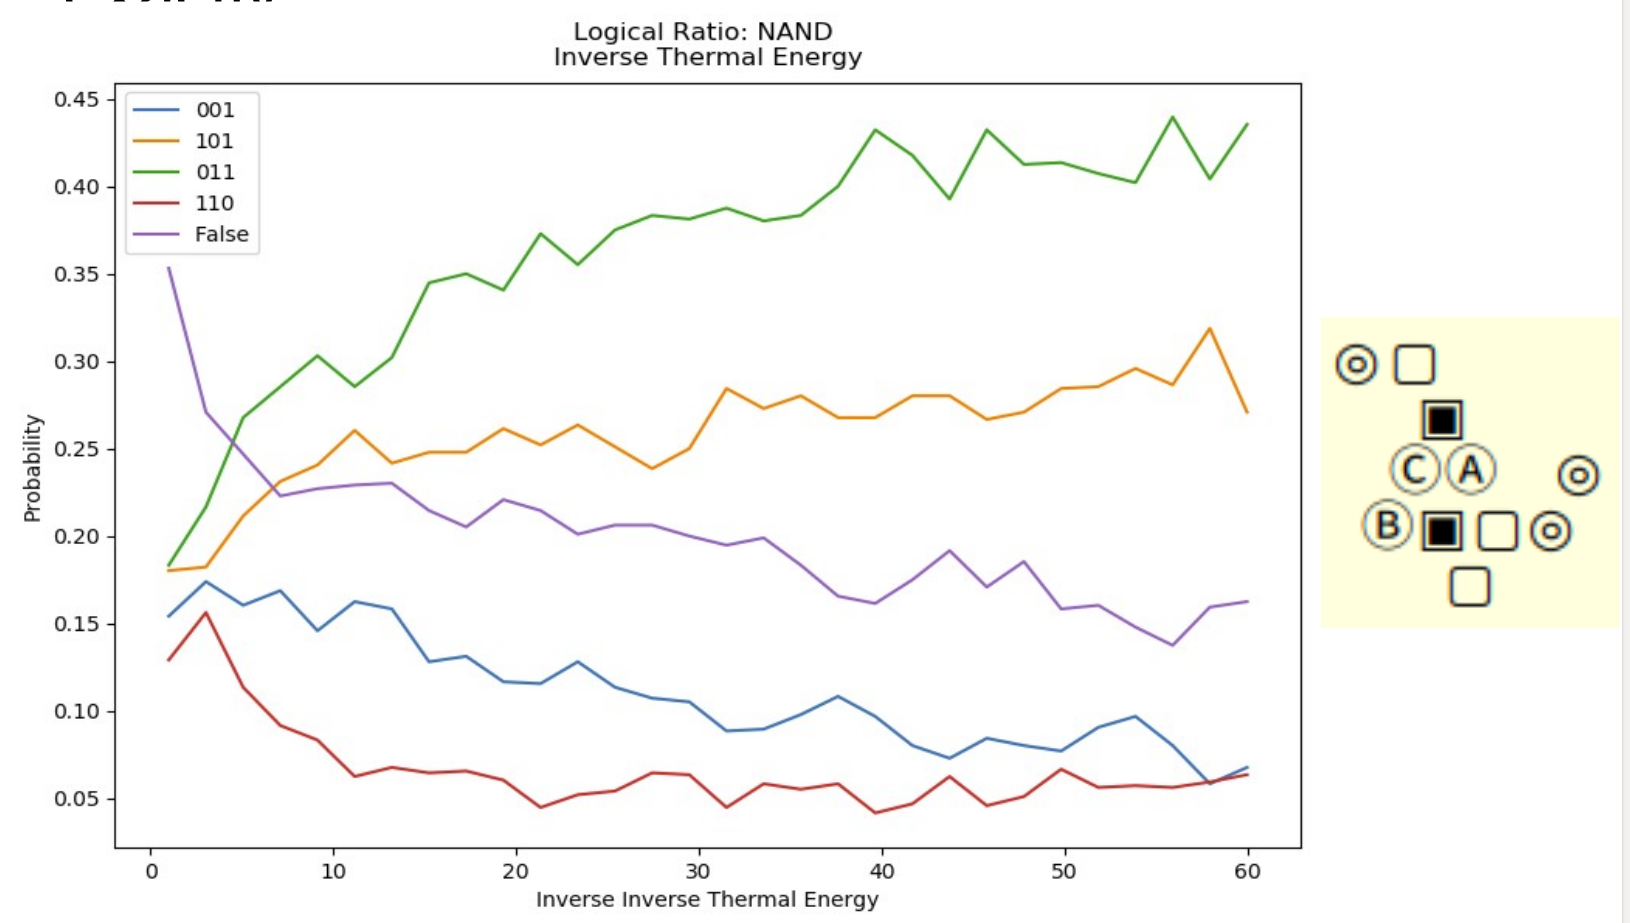}}
	\caption{{\footnotesize BlaBla.}}
	\label{fig:DynOptimalC}
\end{figure} 

We proceed nonetheless to consider the the effect of finely tuning the saturation magnetization $M_S$ of the free islands. Figures~\ref{fig:MsDynOptimalA} and \ref{fig:RevMsDynOptimalA} show how the observed logical probabilities are effected as a function of a scaling parameter multiplying $M_S$ in Eq. (\ref{eq:sLLG}) in the free-floating state. Figure~\ref{fig:MsDynOptimalA} considers a gate where the terminal islands are allowed to evolve freely whereas Figure~\ref{fig:RevMsDynOptimalA} constrains the output island into a $1$-state and monitors how the input islands respond. In both cases, the introduction of this new design flexibility allows to significantly boost both the $LC$ measure and control dispersion in the probability of the individual logical states. We do observe however that the optimal scaling factors are differ significantly between the constrained (Fig.~\ref{fig:MsDynOptimalA}) and unconstrained (Fig.~\ref{fig:RevMsDynOptimalA}) cases. Whereas the former displays optimal operation in accordance with a slight reduction of the free-island $M_S$, the latter displays optimality in the presence of a slight increase of the same. Nonetheless, we claim that this approach demonstrates that sufficient magnetic tunability exists to optimize the logical operation of stray-field-coupled NML gates when exposed to strong thermal effects exciting persistent out-of-equilibrium transient states.

\begin{figure}
	\centerline{\includegraphics[width=6in]{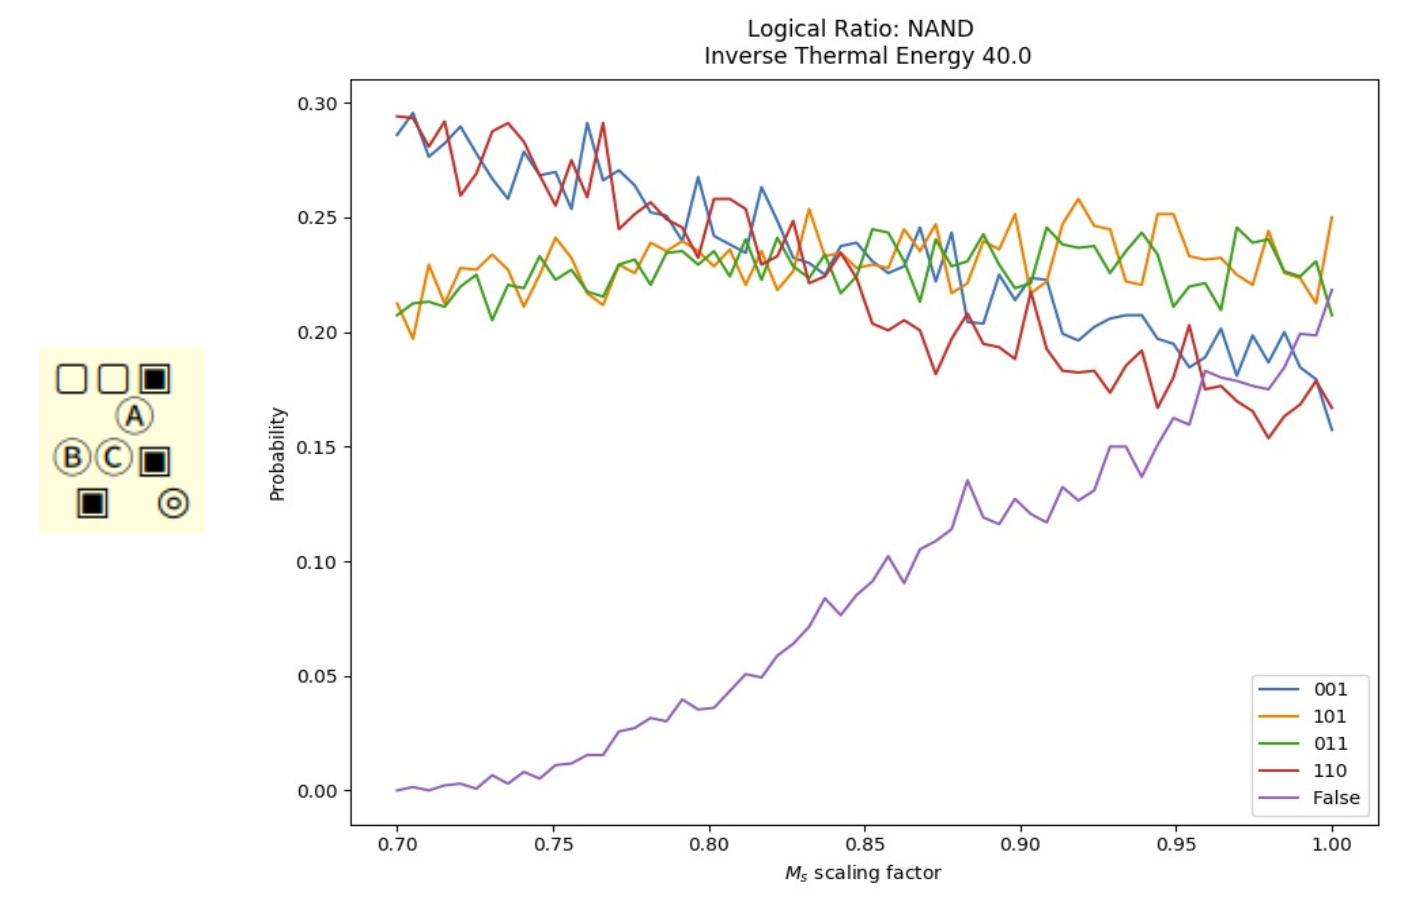}}
	\caption{{\footnotesize BlaBla.}}
	\label{fig:MsDynOptimalA}
\end{figure} 

\begin{figure}
	\centerline{\includegraphics[width=6in]{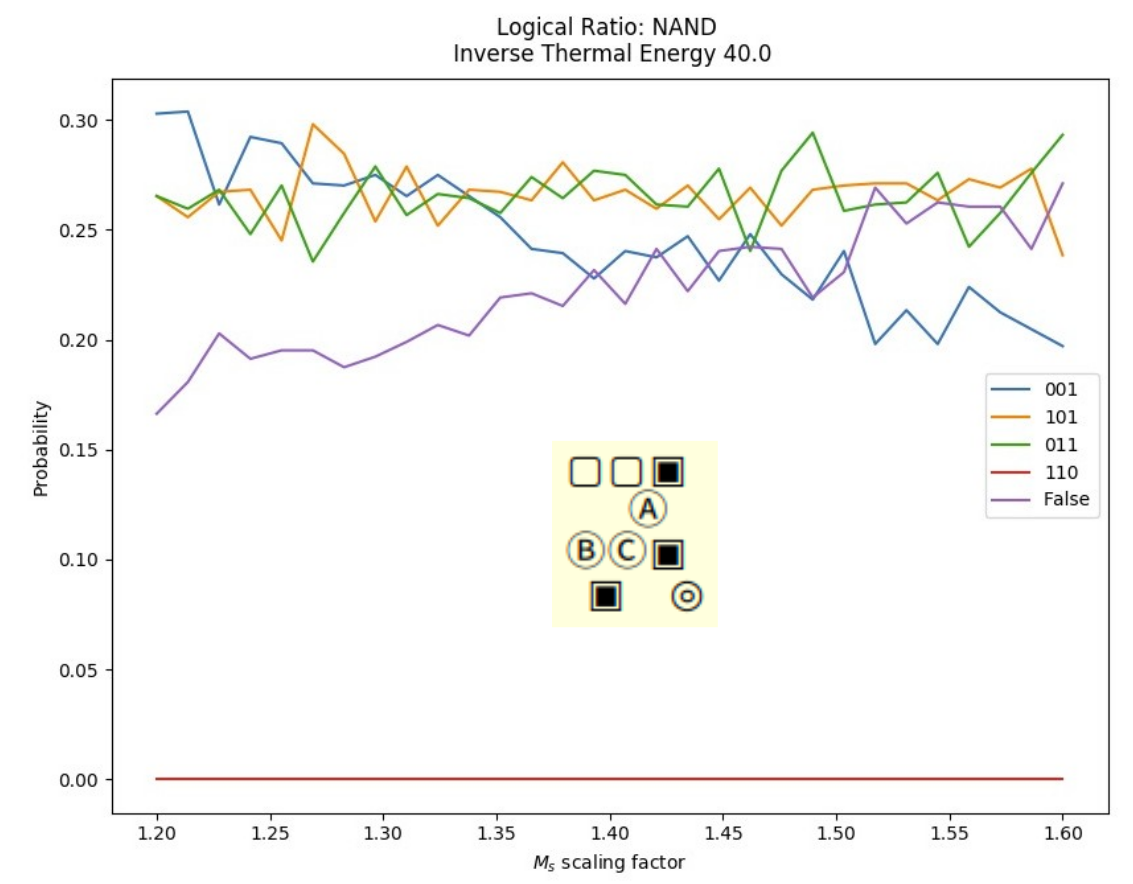}}
	\caption{{\footnotesize BlaBla.}}
	\label{fig:RevMsDynOptimalA}
\end{figure}
