# Supplementary material for: Nanomagnetic Self-Organizing Logic Gates
Source: arXiv:2012.12721 source file (2020-12-23)
Supplement: Supplementary file 2 [file Suppl_ErrorSuppressionDetails.tex]

\subsection{DES model}
The logical correctness is checked after a time $\tau_{\mathrm{check}}$ and, in case of a logically incorrect state, an additional field is applied on each island for a duration of $\tau_{\mathrm{DES}}$. This $\tau_{\mathrm{DES}}$ was chosen as fraction of average switching time of a gate with the ES field applied. For our parameters, this average switching time was 200~ps and $\tau_{\mathrm{DES}}=0.05\tau_{\mathrm{switch}}=$~10~ps. The rate a witch the logic is checked was set to $\tau_{\mathrm{check}}=4\tau_{\mathrm{DES}}=$~40~ps.

For a NAND and NOR gate consisting of input islands A and B, and output island C, these ES field were set at
\begin{eqnarray}
    B_{ES}^{A}(\mathrm{T}) &=& -0.080\bigg[ m_z^B/(\sqrt{3})^3 + m_z^C \bigg]\\
    B_{ES}^{B}(\mathrm{T}) &=& -0.080\bigg[ m_z^A/(\sqrt{3})^3 + m_z^C \bigg]\\
    B_{ES}^{C}(\mathrm{T}) &=& -0.080\bigg[ m_z^A + m_z^B \bigg] \pm 0.049
    \label{eq:ES_nandnor}
\end{eqnarray}
where the $+$sign and $-$sign of Eq.\ (\ref{eq:ES_nandnor}) correspond to the NAND and NOR gate, respectively. $m_z$ denotes the magnetization along the easy axis. The factor $(\sqrt{3})^3$ takes into account that magnetostatic interaction between the input islands is weaker due to the larger distance between these islands as shown in Figure \ref{fig:1_nand_design}(b). For a coupling between islands D and E, these ES field were set at 
\begin{eqnarray}
    B_{ES}^{D}(\mathrm{T}) &=& +0.080\ m_z^E\\
    B_{ES}^{E}(\mathrm{T}) &=& +0.080\ m_z^D
    \label{eq:ES_coup}
\end{eqnarray}
to promote that the magnetization of these islands points in the same direction. 

For a gate consisting of non-interacting islands, for which the logical NAND behavior is totally embedded within the ES scheme, these ES field were set at
\begin{eqnarray}
    B_{ES}^{A}(\mathrm{T}) &=& -0.080\bigg[ m_z^B/(\sqrt{3})^3 + m_z^C \bigg]+0.945H_{{\rm 2sm}}\\
    B_{ES}^{B}(\mathrm{T}) &=& -0.080\bigg[ m_z^A/(\sqrt{3})^3 + m_z^C \bigg]+0.945H_{{\rm 2sm}}\\
    B_{ES}^{C}(\mathrm{T}) &=& -0.080\bigg[ m_z^A + m_z^B \bigg] + 0.038 + 0.945\times2H_{{\rm 2sm}}
    \label{eq:ES_random}
\end{eqnarray}
with $H_{{\rm 2sm}} = 0.019 T$ the bias field obtained from the two-state model. For a coupling between non-interacting islands D and E, these ES field were set at 
\begin{eqnarray}
    B_{ES}^{D}(\mathrm{T}) &=& +0.640\ m_z^E\\
    B_{ES}^{E}(\mathrm{T}) &=& +0.640\ m_z^D.
    \label{eq:ES_randcoup}
\end{eqnarray}

\begin{figure}[H]
	\centerline{\includegraphics[width=\textwidth]{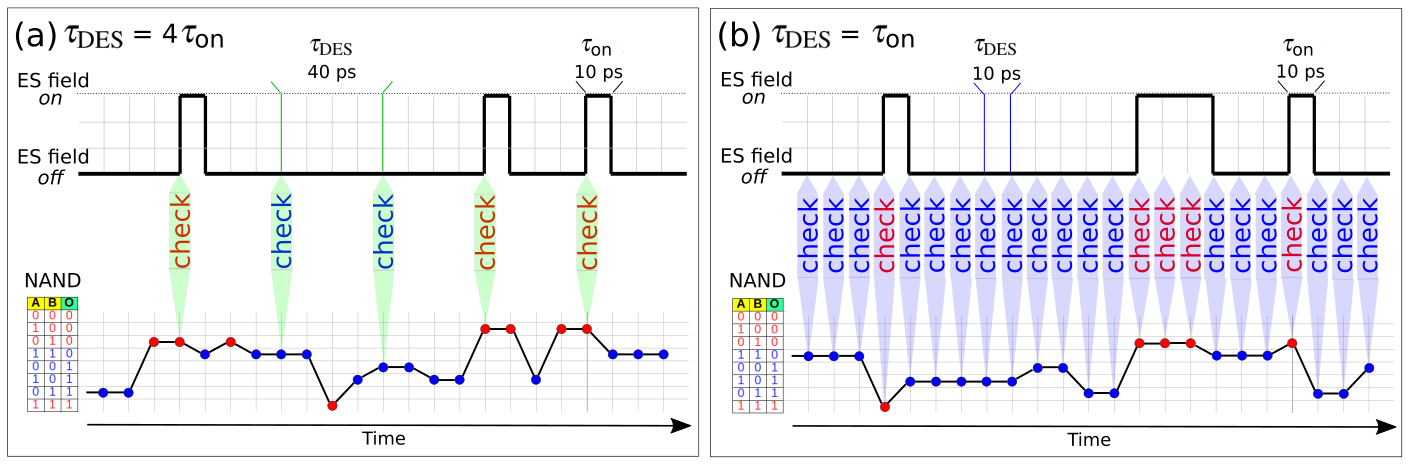}}
	\caption{{\footnotesize {\bf Schematic representation of dynamic error suppression (DES).} {\bf (a)} $\tau_{\mathrm{DES}}$ = 4 $\tau_{\mathrm{on}}$ {\bf (b)} $\tau_{\mathrm{DES}}$ = $\tau_{\mathrm{on}}$.
	}}
	\label{fig:DES}
\end{figure}

\subsection{Coupling between gates}
\jonathan{Pieter?}

\subsection{Possible physical implementation}
Such a DES scheme could be realized by adding an extra hardware layer to the magnetic gate. The state of the nanomagnets can be read out through a magnetic tunnel junction (MTJ) and forward logic can be used detect the incorrect state and drive a correction signal in the form of a spin polarized current to help the incorrectly aligned magnets switch to a logically correct state. A lower power alternative could by realized by making use of voltage controlled magnetic anisotropy (VCmA)\cite{MAR-09,WEI-07} to increase the switching probability of the logical inconsistent island during the $\tau_{\mathrm{DES}}$.
