# Supplementary material for: Nanomagnetic Self-Organizing Logic Gates
Source: arXiv:2012.12721 source file (2020-12-23)
Supplement: Supplementary file 3 [file Suppl_FixedOutput.tex]

Due to the additional degrees of freedom of the macrospin model as compared to the two-state model, the magnetic moment of the bias island has to be tuned in order to recover the balancedness. The tuning of the relative bias was shown in Fig. 1(d) for a NAND gate with a free output. However, gates with a fixed output are required for solving factorization problems, i.e.\ to decompose a \emph{fixed} output number into its (prime)factors. Fixing the output affects the state space, which results in another tuning of the relative bias field (see Fig. \ref{fig:fixedout}).

The probability distributions of a SO-NAND gate and a SO-XNOR gate with fixed output are shown in Fig. \ref{fig:fixedout}(b) and (c), respectively. 

\begin{figure}[H]
	\centerline{\includegraphics[width=5in]{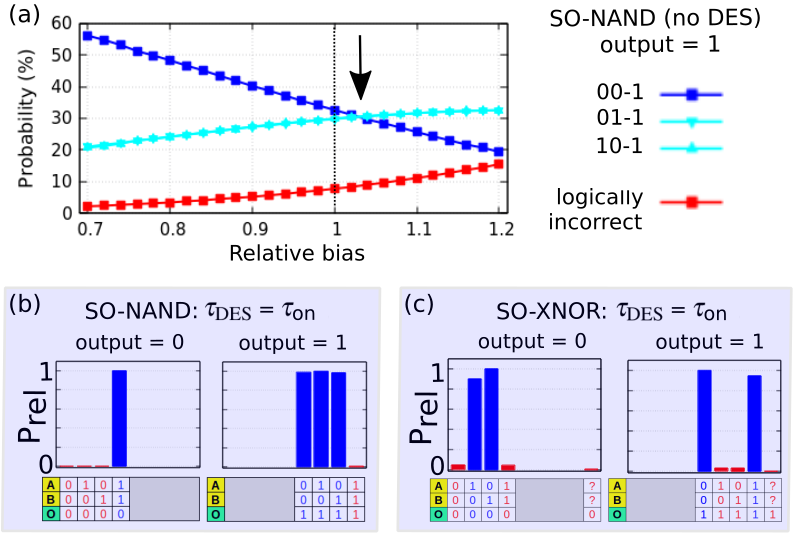}}
	\caption{{\footnotesize {\bf SO-gates with a fixed output.} {\bf (a)} The balancedness of a SO-NAND gate with output $1$ is recovered at a relative bias strength of 1.04, corresponding to the point where the probabilities of all logically correct states are equal, as indicated by the arrow. The two-state model corresponds to relative bias = 1. {\bf (b)} Probability distributions of a SO-NAND gate with fixed output {\bf (c)} Probability distributions of a SO-XNOR gate with fixed output.}}
	\label{fig:fixedout}
\end{figure}
