# Supplementary material for: Nanomagnetic Self-Organizing Logic Gates
Source: arXiv:2012.12721 source file (2020-12-23)
Supplement: Supplementary file 4 [file Suppl_NoteOnP-BitScaling.tex]

As mentioned in the main text, the p-bit prime factorization demonstration~\cite{borders2019integer} required that the magnetic state of every sMTJ be read via magnetoresistive measurements on a timescale which scales inversely proportionately to the number of islands one wishes to have coupled. Assuming a network of $N$ coupled elements of which a subset $N_T$ is used to define the binary inputs one wishes to solve for~\footnote{In the case of a sum factorization operation attempting to obtain all pairs of 3-bit numbers whose sum is consistent with a given 4-bit output one must necessarily have $N\geq 6$ as at least one sMTJ is needed to represent each significant bit of the operation. In such a setting one would accordingly have $N_T=6$.}, the dynamics of the system must perform a Gibbs sampling of $2^{N_T}$ possible input states. Due to the exponential scaling of such a solution space, one must engineer for rapidly fluctuating sMTJ elements whose natural switching timescale $\tau_{\mathrm{switch}}$ is such that, relative to the maximum total operation time $\tau_{\mathrm{tot}}$ one has at disposal, the condition $\tau_{\mathrm{tot}}/\tau_{\mathrm{switch}}\gg 2^{N_T}/N_T$ holds. The origin of the $1/N_T$ contribution to the scaling results from the notion that the switching probability of any one free element can be roughly considered Poisson-distributed with mean switching time $\tau_{\mathrm{switch}}/N_T$. 

The number $N$ of free sMTJ elements used in such a construction can in principle be larger than $N_T$ depending on how the current biasings are constructed to define the Boolean problem of interest. This means that the intermediate three-step operation of magnetoresistive state read, digital elaboration of the biasing current intensities, and their application, must take place on a timescale $\tau_{\mathrm{adjust}} \ll \tau_{\mathrm{switch}}/N$ to ensure proper performance. To quantify the magnitude of these limitations, let us assume a natural sMTJ switching time of $\tau_{\mathrm{switch}}\simeq 1,\mu\mathrm{s}$ whose read/adjust operation can somehow be performed on a nanosecond timescale. Let us further assume that the Boolean problem of interest is ideally constructed ($N=N_T$). This places the fundamental limit $N_T\ll\tau_{\mathrm{switch}}/\tau_{\mathrm{adjust}}\sim 10^3 $ on the amount of significant bits one can operate on. One can of course engineer the sMTJ elements to have even slower natural switching times. For $\tau_{\mathrm{switch}}\sim 10\,\mu\mathrm{s}$ one might attempt to execute the reversion of an elliptic curve encryption operation by taking a public key as a fixed output and solving for its 256-bit private key pair. The total time taken to perform such an operation can be estimated, resulting in a gargantuan $\tau_{\mathrm{tot}}\simeq (2^{256}/256)\tau_{\mathrm{switch}}\sim 10^{69}\mathrm{s}$.)
