# Supplementary material for: Nanomagnetic Self-Organizing Logic Gates
Source: arXiv:2012.12721 source file (2020-12-23)
Supplement: Supplementary file 5 [file Suppl_StaticAnalysis.tex]

Logic gates are defined by their truth tables consisting of $\lambda_q,\,q=1,...,2^{N_{\mathrm{in}}}$ allowed combinations of simultaneous input/output terminal states. We will denote the set of allowed logical combinations as $\Lambda$. By fixing a certain logical function we wish to reproduce, at each iteration of terminal island labels we can assign an overall logical label $\lambda_s$ to each spin-flip state $\sigma_s$ if the magnetic state of the terminal island magnetizations replicates one of the input-output conditions defined by the logic function one is trying to emulate. Otherwise we will say that $\sigma_s\notin\Lambda$. The logical consistency $LC$ of the island configuration and terminal permutation chosen can then be defined as:

\begin{equation}
LC \equiv \frac{\sum_{s || \sigma_s\in\Lambda}\exp^{-\beta \epsilon(\sigma_s)}}{\sum_s \exp^{-\beta \epsilon(\sigma_s)}}.
\end{equation}  

Similarly we can compute the relative Boltzmann probability of all $\sigma_s$ spin-flip states satisfying a specific logical condition $\lambda_q$:

\begin{equation}
P[\lambda_q] = \frac{\sum_{s || \lambda_s=\lambda_q}\exp^{-\beta \epsilon(\sigma_s)}}{\sum_s \exp^{-\beta \epsilon(\sigma_s)}}.
\end{equation}
Well-Balancedness $WB$ can then be defined as the variance of the Boltzmann-averaged probabilities across all logical conditions:

\begin{equation}
WB \equiv \mathrm{var}(\{P[\lambda_q]\}).
\end{equation}

For NAND logic, where four distinct three-terminal combination are allowed out of a total of eight (see Table -reference-), it will always be the case that in the limit of large temperatures ($\beta\ll\epsilon(\sigma_{2^{(N-N_{\mathrm{fix}})}})$) $LC = 0.5$ and $WB = 0$. This must necessarily be so as in such a limit all terminal island combinations are equally likely ($P[\lambda_q]=0.125\;\forall q$). We wish to find gate configurations that maximize $LC$ while keeping $WB$ minimal across as wide a thermal energy range as possible. In Figure~\ref{fig:TriGate}, a simple gate design is used to highlight the temperature dependence of $LC$ and $WB$ on thermal energy. The gate highlights an example of a sub-optimal gate due to the fact that though it retains relatively high $LC$ values across an initial range of thermal energies, the Boltzmann probabilities of the individual logically allowed states are spread across a wide range throughout the range.

\begin{figure}[H]
	\centerline{\includegraphics[width=6in]{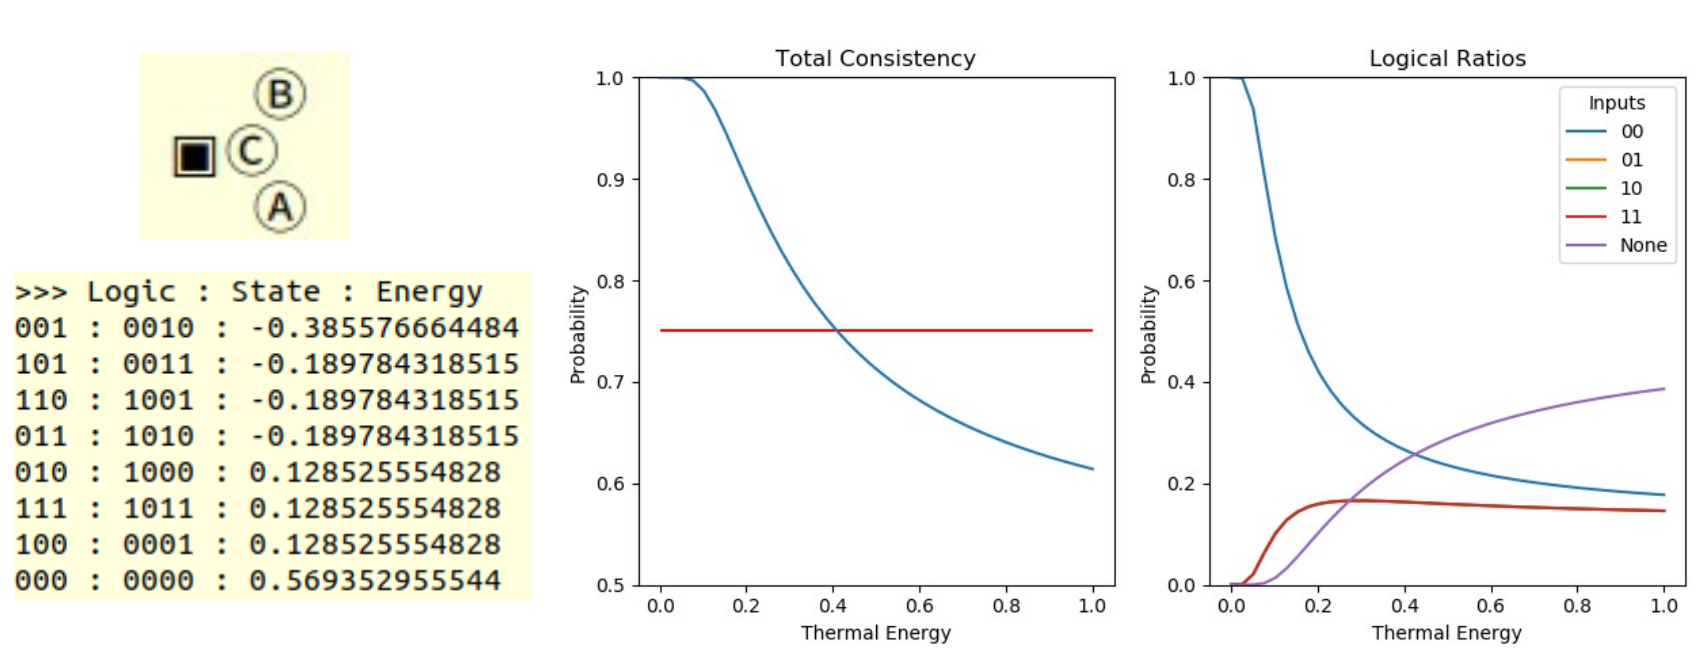}}
	\caption{{\footnotesize Simple NAND gate design highlighting the typical dropoff of logical consistency and lowering of well-blanacedness as a function of increasing temperature. This gate would not be considered a good gate design due to the wide disparity of Boltzmann probabilities among the different logically allowed terminal island states. The table lists all eight possible spin-flip states $\sigma_s$ along with their respective logical labels and their relative energies.}}
	\label{fig:TriGate}
\end{figure} 

The three best performing gates obtained from our brute force search are shown in Figures~\ref{fig:OptimalA},~\ref{fig:OptimalB}, and~\ref{fig:OptimalC}. As expected, the $LC$ values drop off at high thermal energies for all of them. A significant thermal range exists, however, where values of $LC>0.75$. The gate designs proposed exhibit an exceptional balancedness due to the Boltzmann probabilities of each allowed logical state effectively equaling each other even though the ensembles rarely ever exhibit a degeneracy of states like the well-balanced gate mentioned in Section~2. Having massively narrowed down our search to these three potential NAND gate designs, we proceeded to study each dynamically to assess whether these static results hold in the presence of thermal excitations.

\begin{figure}[H]
	\centerline{\includegraphics[width=6in]{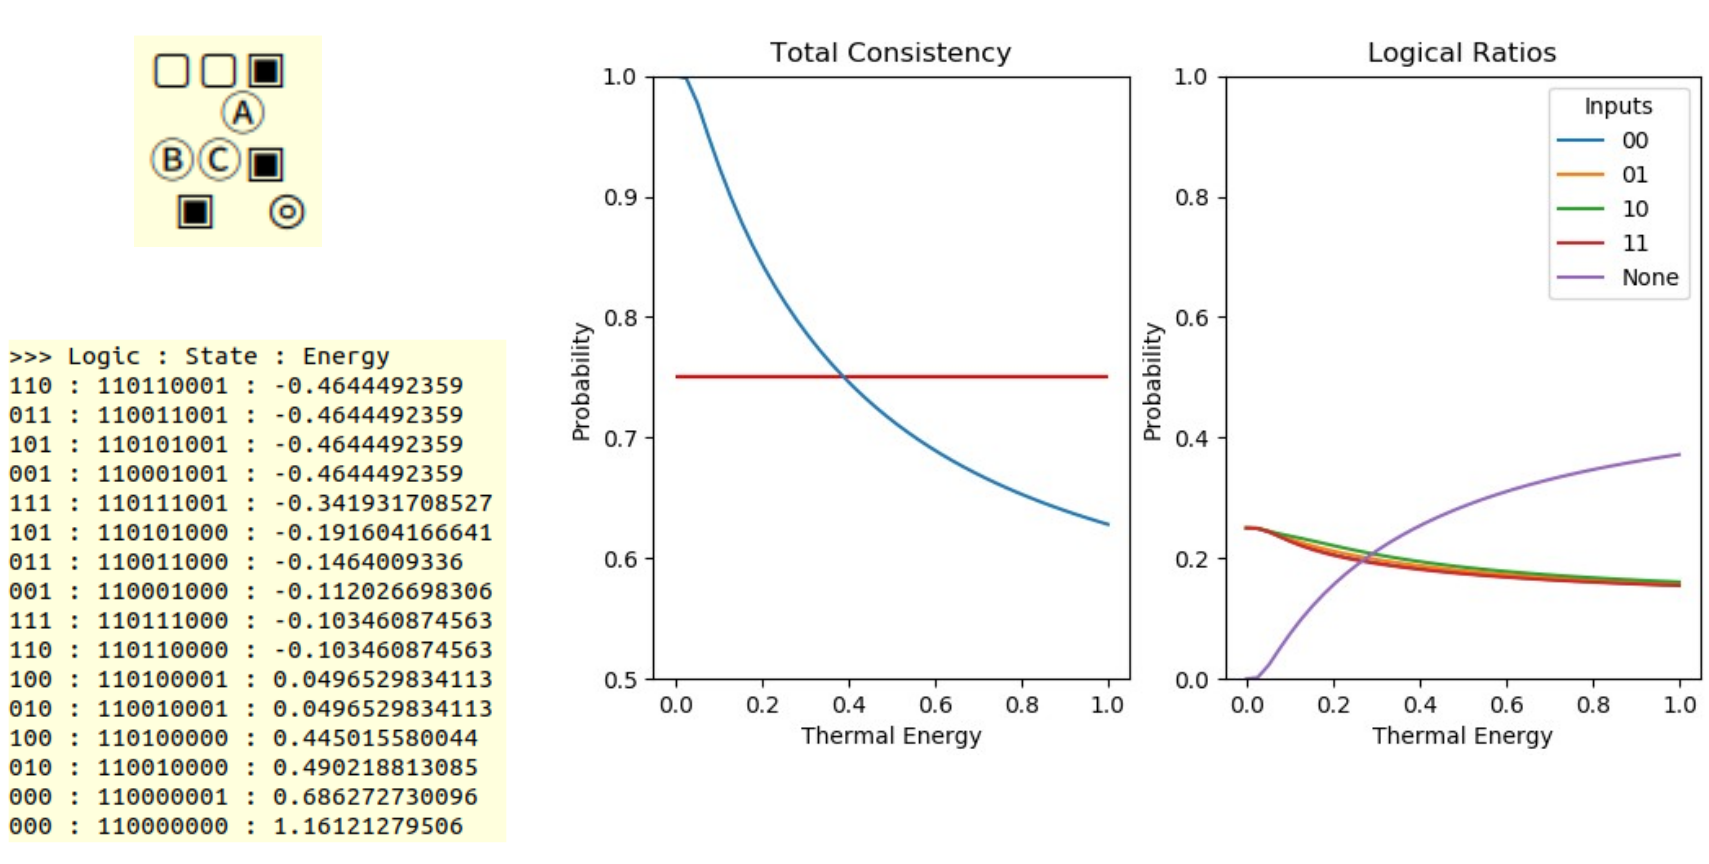}}
	\caption{{\footnotesize BlaBla.}}
	\label{fig:OptimalA}
\end{figure} 

\begin{figure}[H]
	\centerline{\includegraphics[width=6in]{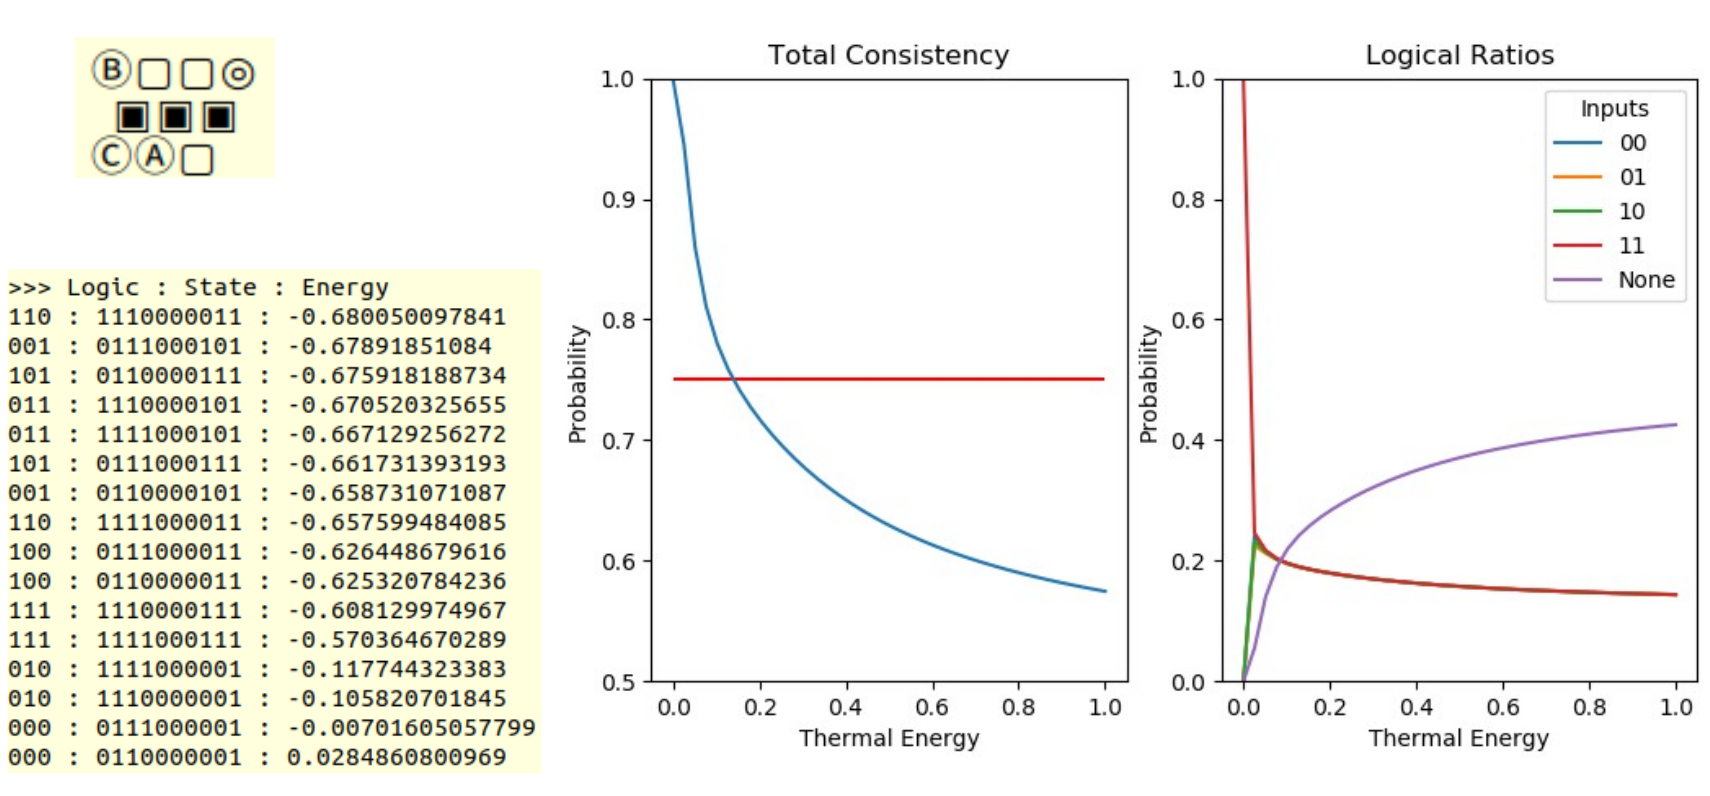}}
	\caption{{\footnotesize BlaBla.}}
	\label{fig:OptimalB}
\end{figure} 

\begin{figure}[H]
	\centerline{\includegraphics[width=6in]{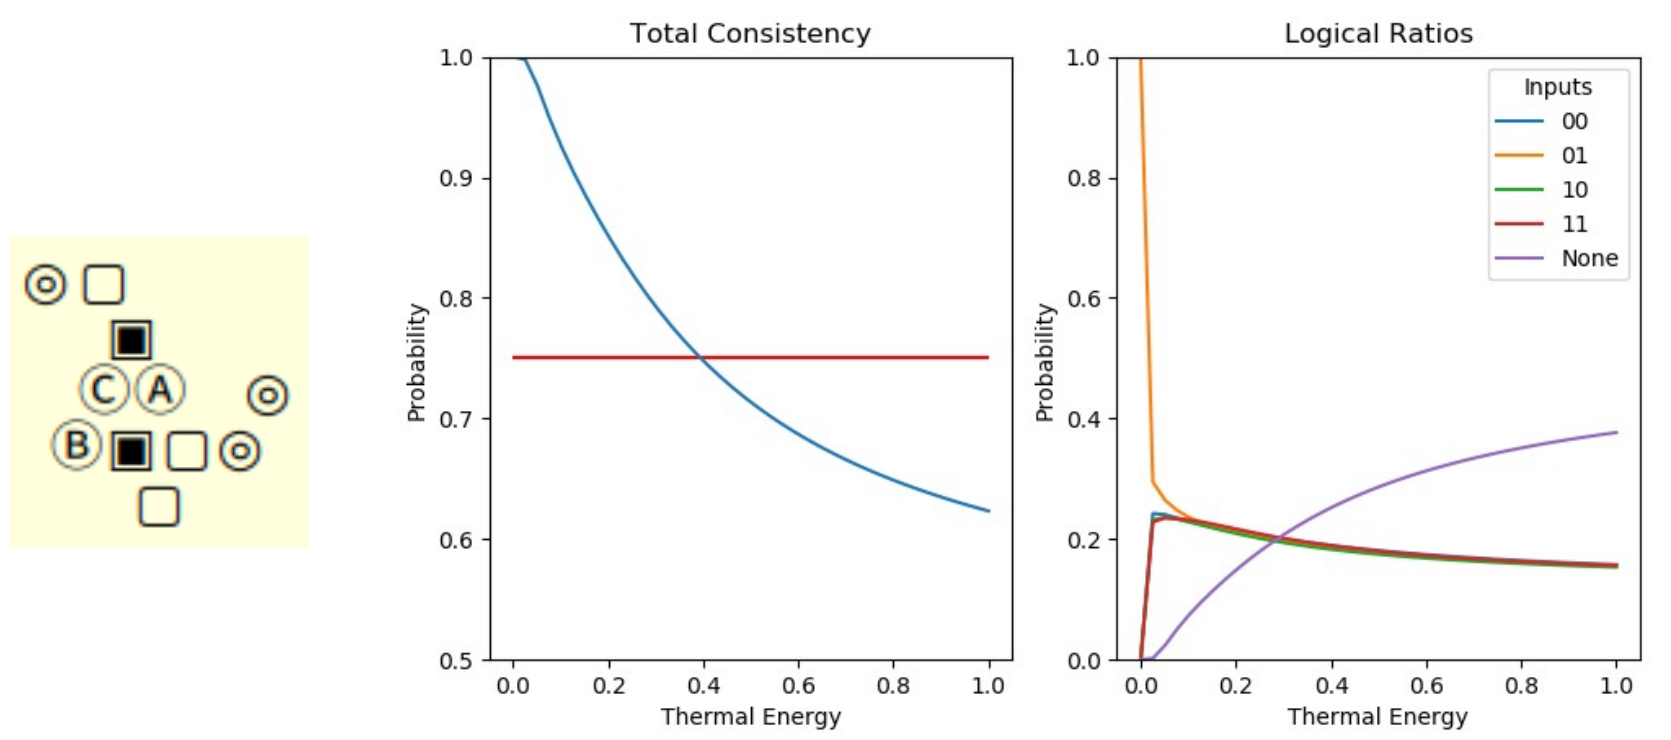}}
	\caption{{\footnotesize BlaBla.}}
	\label{fig:OptimalC}
\end{figure}
