# Supplementary material for: Nanomagnetic Self-Organizing Logic Gates
Source: arXiv:2012.12721 source file (2020-12-23)
Supplement: Supplementary file 6 [file 08_additionalInfo.tex]

To include, in this order: \textbf{Accession codes} (where applicable); \textbf{Competing interests} (mandatory statement). 

The corresponding author is responsible for submitting a \href{http://www.nature.com/srep/policies/index.html#competing}{competing interests statement} on behalf of all authors of the paper. This statement must be included in the submitted article file.

\begin{figure}[ht]
\centering
\includegraphics[width=\linewidth]{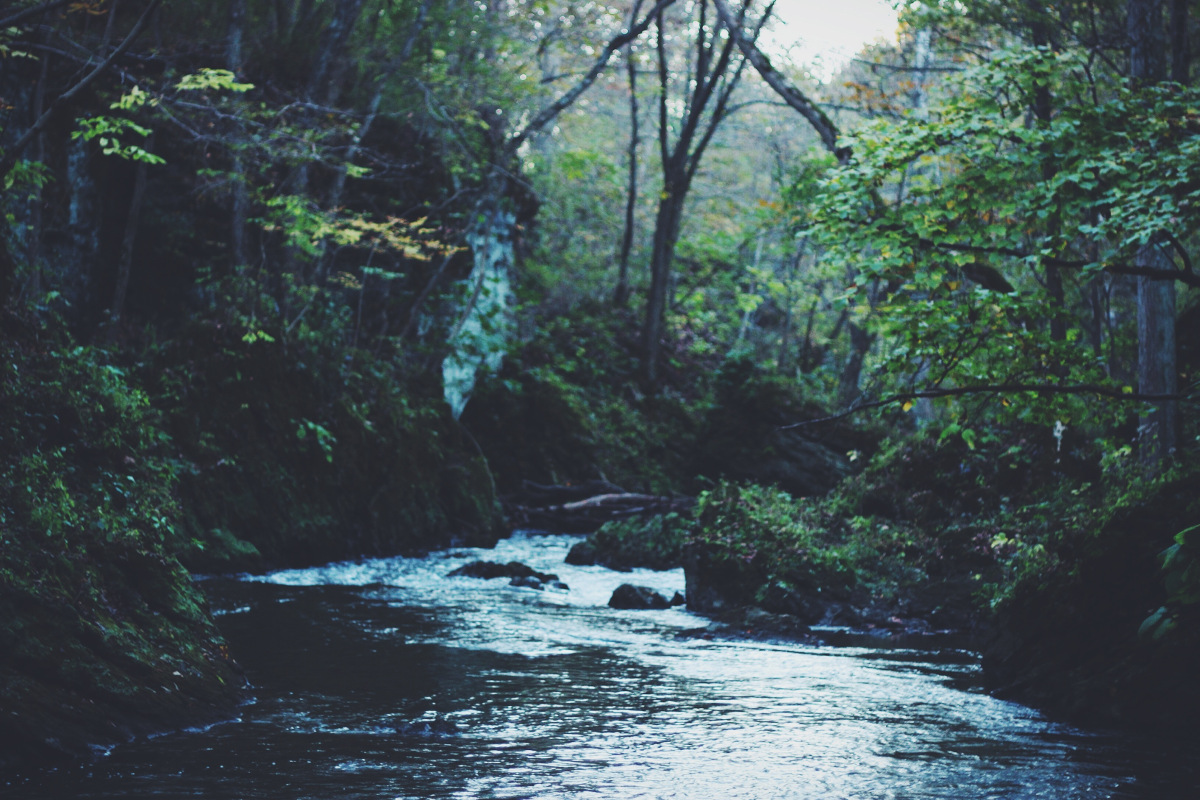}
\caption{Legend (350 words max). Example legend text.}
\label{fig:stream}
\end{figure}

\begin{table}[ht]
\centering
\begin{tabular}{|l|l|l|}
\hline
Condition & n & p \\
\hline
A & 5 & 0.1 \\
\hline
B & 10 & 0.01 \\
\hline
\end{tabular}
\caption{\label{tab:example}Legend (350 words max). Example legend text.}
\end{table}

Figures and tables can be referenced in LaTeX using the ref command, e.g. Figure \ref{fig:stream} and Table \ref{tab:example}.
