# Supplementary material for: Nanomagnetic Self-Organizing Logic Gates
Source: arXiv:2012.12721 source file (2020-12-23)
Supplement: Supplementary file 7 [file Suppl_Influence.tex]

As compared to the results of the two-state model, the  additional degrees of freedom in the macrospin model negatively impact the balancedness of the gate.

The balancedness can be recovered by tuning the magnetic moment of the bias island, as shown in Fig. 
 \ref{fig:1_nand_design}(d).
 Figure \ref{fig:influence}, shows that this tuning is robust as a $20\%$ change in the damping,  temperature, or uniaxial anisotropy constant of our system only result in a 2\% change of the required bias to recover the balancedness.

\begin{figure}[H]
	\centerline{\includegraphics[width=\textwidth]{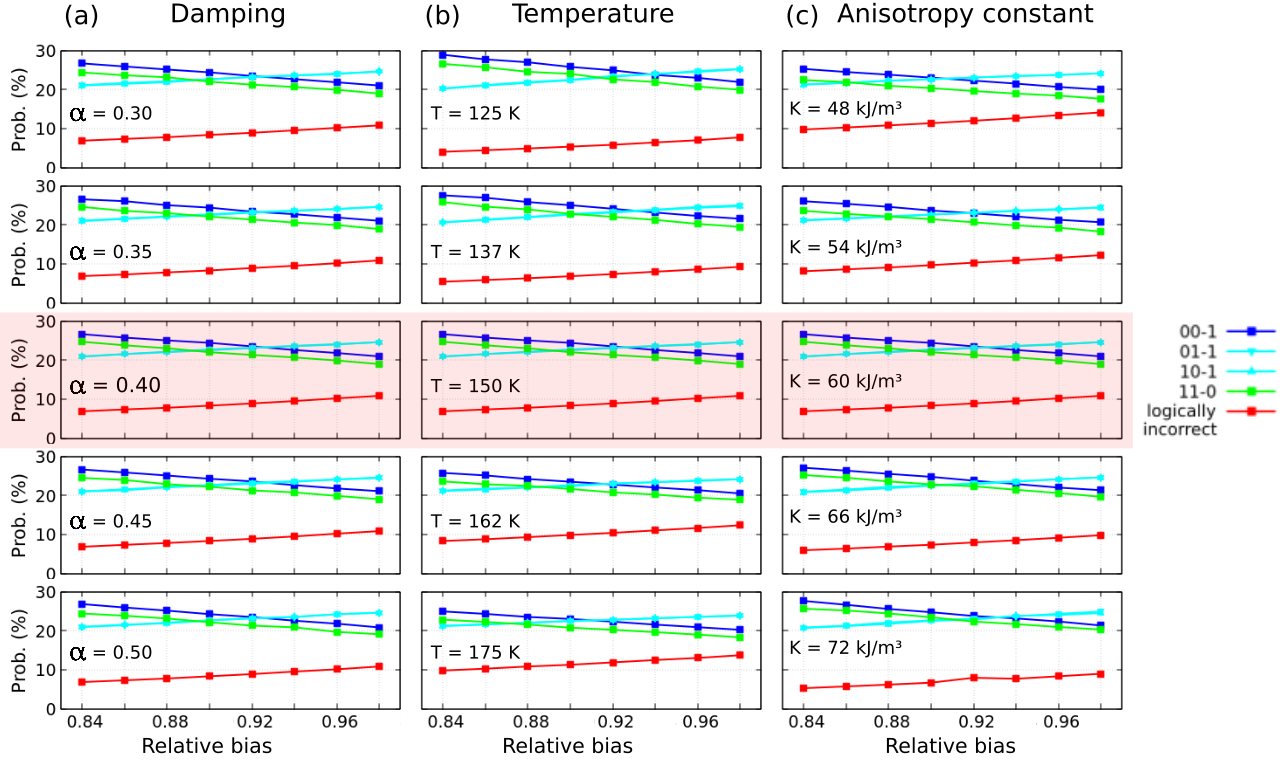}}
	\caption{{\footnotesize 
	Probabilities for the logic states, obtained with the macrospin model for different relative bias strengths for varying \textbf{(a)} damping, \textbf{(b)} temperature, and \textbf{(c)} anisotropy constant. The highlighted region corresponds to the simulation parameters of the main paper.}}
	\label{fig:influence}
\end{figure}
