# Supplementary material for: Nanomagnetic Self-Organizing Logic Gates
Source: arXiv:2012.12721 ancillary file (2020-12-23)
Supplement: Supplementary file 8 [file supp_nanomagnetic_logic_paper.pdf]

# Supplemental materials: Nanomagnetic Self-Organizing Logic Gates

Pieter Gypens<sup>1</sup>, Jonathan Leliaert<sup>1</sup>, Massimiliano Di Ventra<sup>3</sup>, Bartel Van Waeyenberge<sup>1</sup>, and Daniele Pinna<sup>2,4</sup>

<sup>1</sup>Dept. of Solid State Sciences, Ghent University, Belgium

<sup>2</sup>Dept. of Physics, Johannes Gutenberg Universität, Mainz, Germany

<sup>3</sup>Department of Physics, University of California San Diego, La Jolla, USA

<sup>4</sup>Peter Grünberg Institute and Institute for Advanced Simulation, Forschungszentrum, Jülich, Germany

## 1 SO-NAND gate with fixed output

Due to the additional degrees of freedom of the macrospin model as compared to the two-state model, the magnetic moment of the bias island has to be tuned in order to recover the balancedness. The tuning of the relative bias was shown in Fig. 2(c) for a SO-NAND gate with a free output. However, gates with a fixed output are required for solving factorization problems, i.e. to decompose a *fixed* output number into its (prime)factors. Fixing the output affects the state space, which results in a different value of the relative bias field – see Fig. S1(a).

The state probability distributions of a SO-NAND gate and a SO-XNOR gate with fixed output are shown in Fig. S1(b) and (c), respectively.

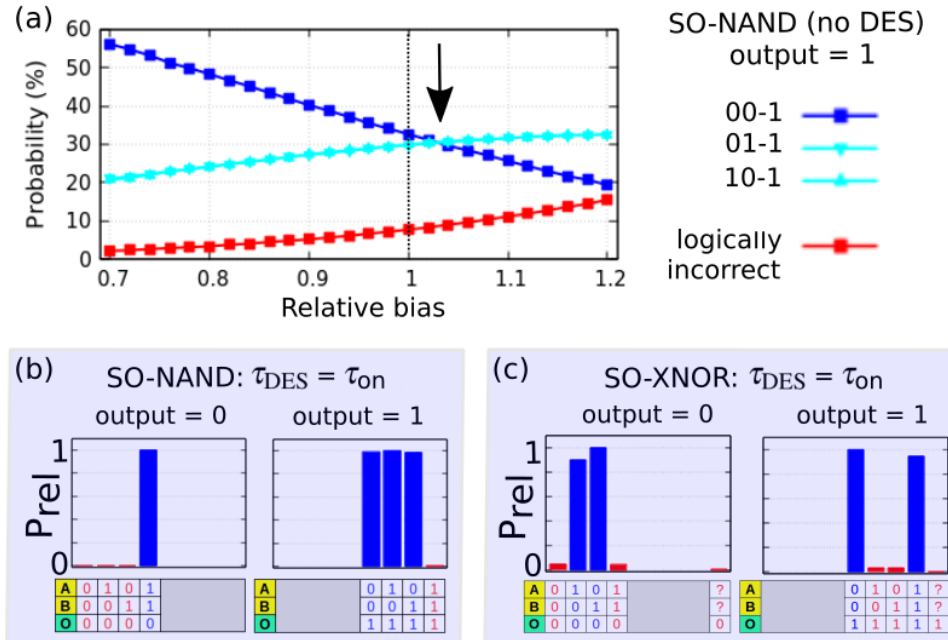

**Figure S1. SO-gates with a fixed output.** (a) The balancedness of a SO-NAND gate with output 1 is recovered at a relative bias strength of 1.04, corresponding to the point where the probabilities of all logically correct states are equal, as indicated by the arrow. The two-state model corresponds to relative bias = 1. (b) State probability distributions of a SO-NAND gate with fixed output.  $P_{rel}$  is the probability relative to the most likely logical state. (c) State probability distributions of a SO-XNOR gate with fixed output.

## 2 Robustness assessment of gate balancedness

As compared to the results of the two-state model, the additional degrees of freedom in the macrospin model negatively impact the balancedness of the gate.

The balancedness can be recovered by tuning the magnetic moment of the bias island, as shown in Fig. 2(c). Figure S2, shows that this tuning is robust as a 20% change in the damping, temperature, or uniaxial anisotropy constant of our system only result in a 2% change of the required bias to recover the balancedness.

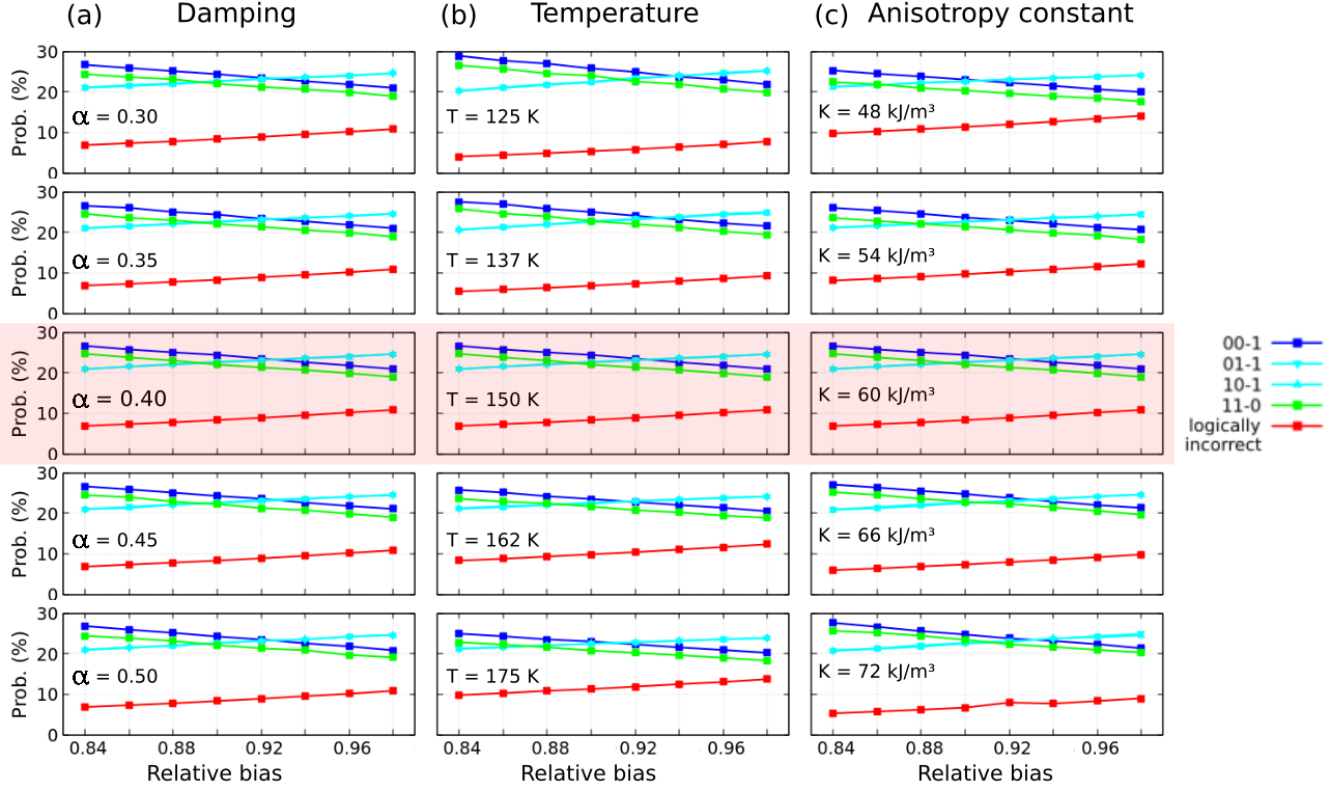

**Figure S2.** Probabilities for the logical states, obtained with the macrospin model for different relative bias strengths for varying (a) damping, (b) temperature, and (c) anisotropy constant. The highlighted region corresponds to the simulation parameters of the main paper.

## 3 Dynamic Error Suppression (DES) scheme

### 3.1 DES model

As shown in Fig. S3, the logical correctness is checked after a time  $\tau_{DES}$  and, in case of a logically incorrect state, an additional field is applied on each island for a duration of  $\tau_{on}$ . This  $\tau_{on}$  was chosen as fraction of the average time of a gate to switch from the logically incorrect 111-state to a logically correct state with the ES field applied [in Eq. (S1)–(S3), all  $m_z$  were set at +1]. For our parameters, this average switching time was  $\tau_{switch} = 200$  ps and  $\tau_{on} = 0.05\tau_{switch} = 10$  ps.

For a NAND and NOR gate consisting of input islands A and B, and output island C, these ES field were set at

$$B_{ES}^A(T) = -0.080 \left[ m_z^B / (\sqrt{3})^3 + m_z^C \right] \quad (S1)$$

$$B_{ES}^B(T) = -0.080 \left[ m_z^A / (\sqrt{3})^3 + m_z^C \right] \quad (S2)$$

$$B_{ES}^C(T) = -0.080 \left[ m_z^A + m_z^B \right] \pm 0.049 \quad (S3)$$

where the +sign and −sign of Eq. (S3) correspond to the NAND and NOR gate, respectively.  $m_z$  denotes the magnetization along the easy axis. The factor  $(\sqrt{3})^3$  takes into account that magnetostatic interaction between the input islands is weaker due to the larger distance between these islands as shown in Fig. 2(a). For a coupling between islands D and E, these ES field were

34 set at

$$B_{ES}^D(T) = +0.080 m_z^E \quad (S4)$$

$$B_{ES}^E(T) = +0.080 m_z^D \quad (S5)$$

35 to promote that the magnetization of these islands points in the same direction.

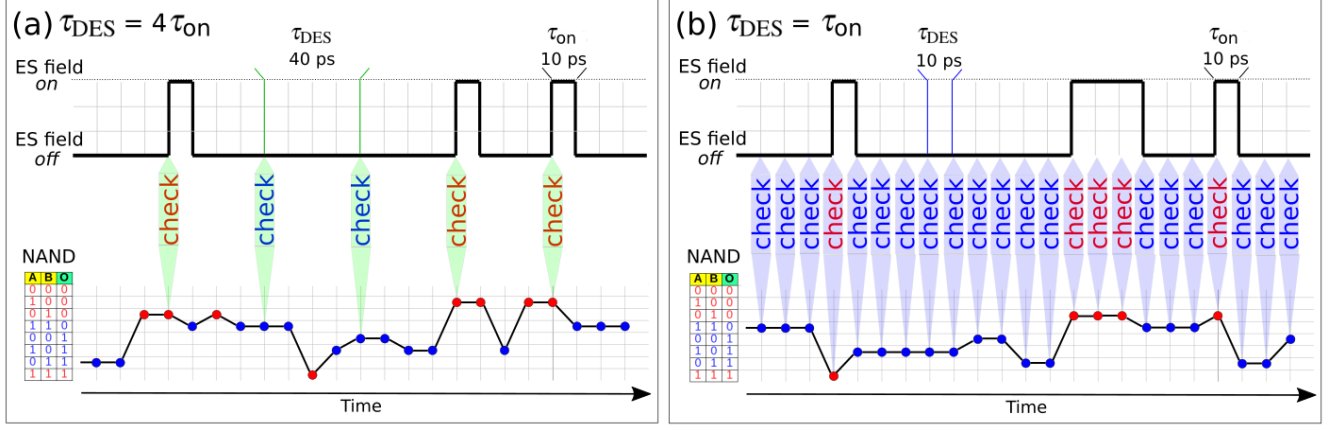

**Figure S3.** Schematic representation of dynamic error suppression (DES). (a)  $\tau_{DES} = 4 \tau_{on}$ . (b)  $\tau_{DES} = \tau_{on}$ .

### 3.2 Possible physical implementation

Such a DES scheme could be realized by adding an extra hardware layer to the magnetic gate. The state of the nanomagnets can be read out through a magnetic tunnel junction (MTJ) and forward logic can be used to detect the incorrect state and drive a correction signal in the form of a spin polarized current to help the incorrectly aligned magnets switch to a logically correct state. A lower power alternative could be realized by making use of voltage controlled magnetic anisotropy (VCMA)<sup>1,2</sup> to increase the switching probability of the logical inconsistent island during the  $\tau_{DES}$ .

## References

1. Maruyama, T. *et al.* Large voltage-induced magnetic anisotropy change in a few atomic layers of iron. *Nat. Nanotechnol.* **4**, 158–161 (2009).
2. Weisheit, M. *et al.* Electric field-induced modification of magnetism in thin-film ferromagnets. *Science* **315**, 349–351 (2007).
